# Supplementary material for: Knowledge is Power: Harnessing Large Language Models for Enhanced Cognitive Diagnosis
Source: arXiv:2502.05556 source file (2025-02-08)
Supplement: Supplementary file 1 [file appendix.tex]

\clearpage
\begin{figure*}[!htb]
  \centering
  \includegraphics[width=0.95\linewidth]{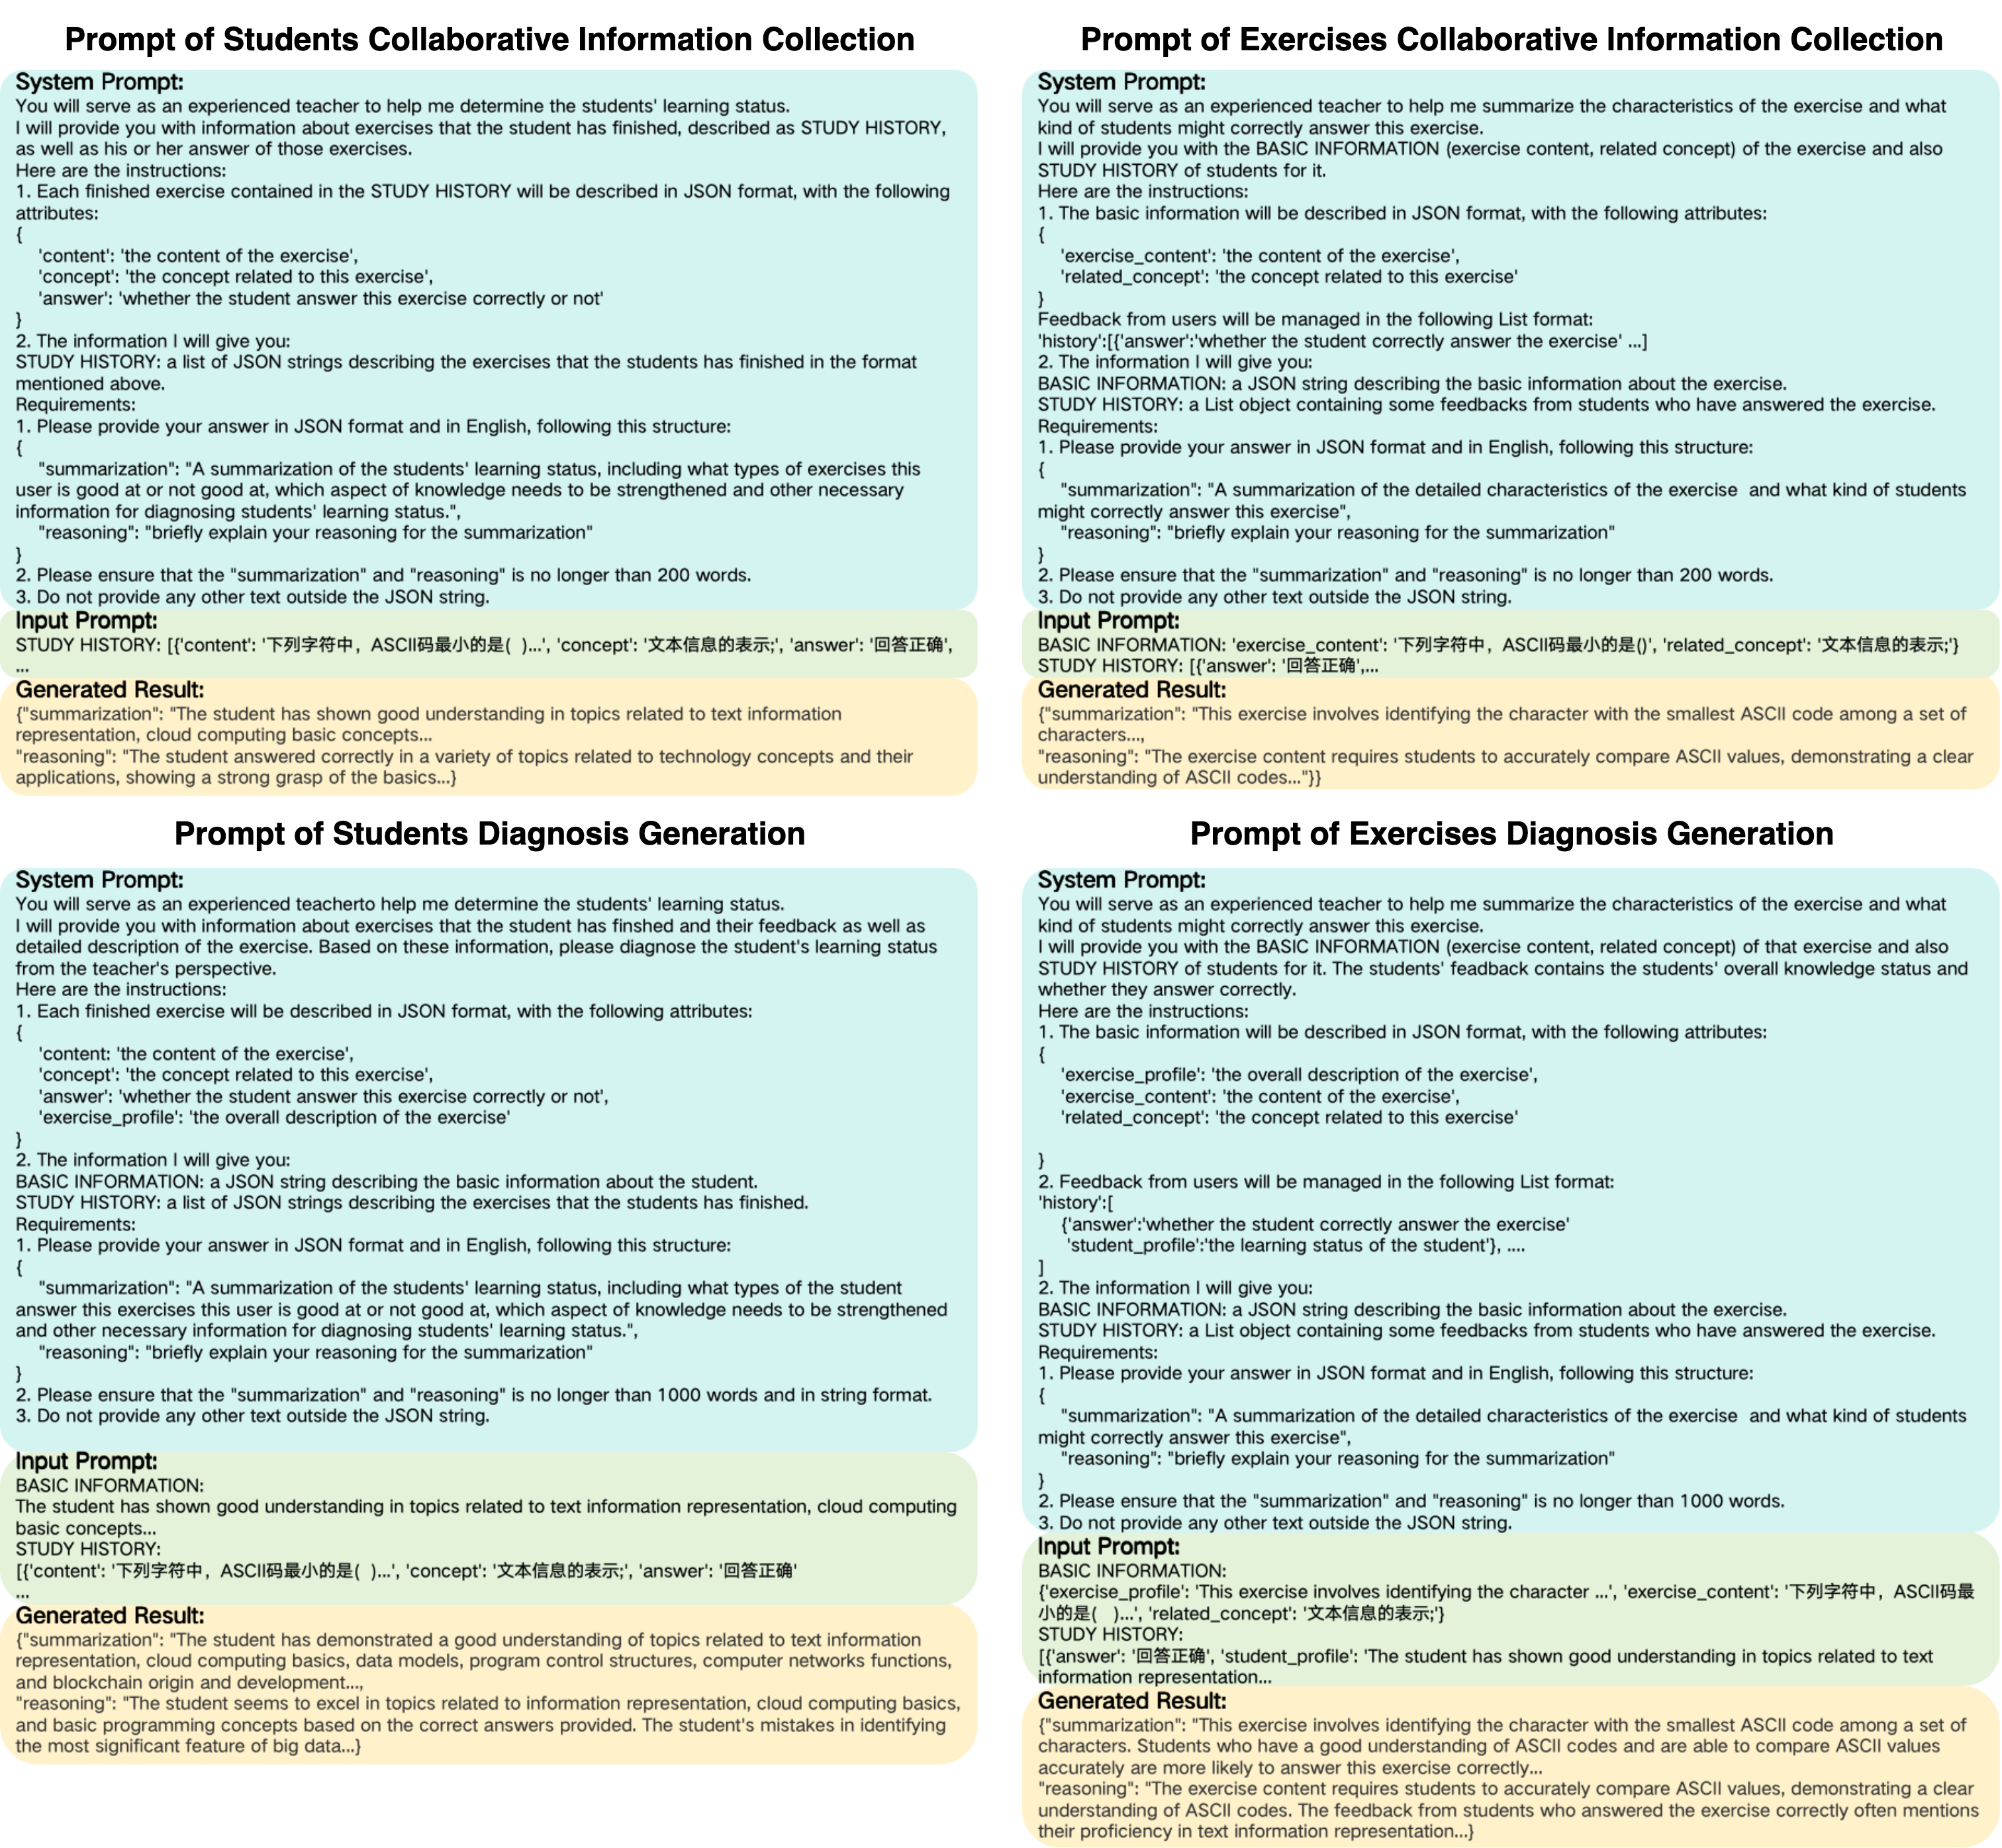}
  \caption{The example of used prompts in LLMs Diagnosis. The Chinese in the input prompt is the exercise content and related knowledge concepts of the PTADisc dataset.}
\label{fig: prompt}
\end{figure*}

\begin{figure*}[!htb]
  \centering
  \includegraphics[width=0.85\linewidth]{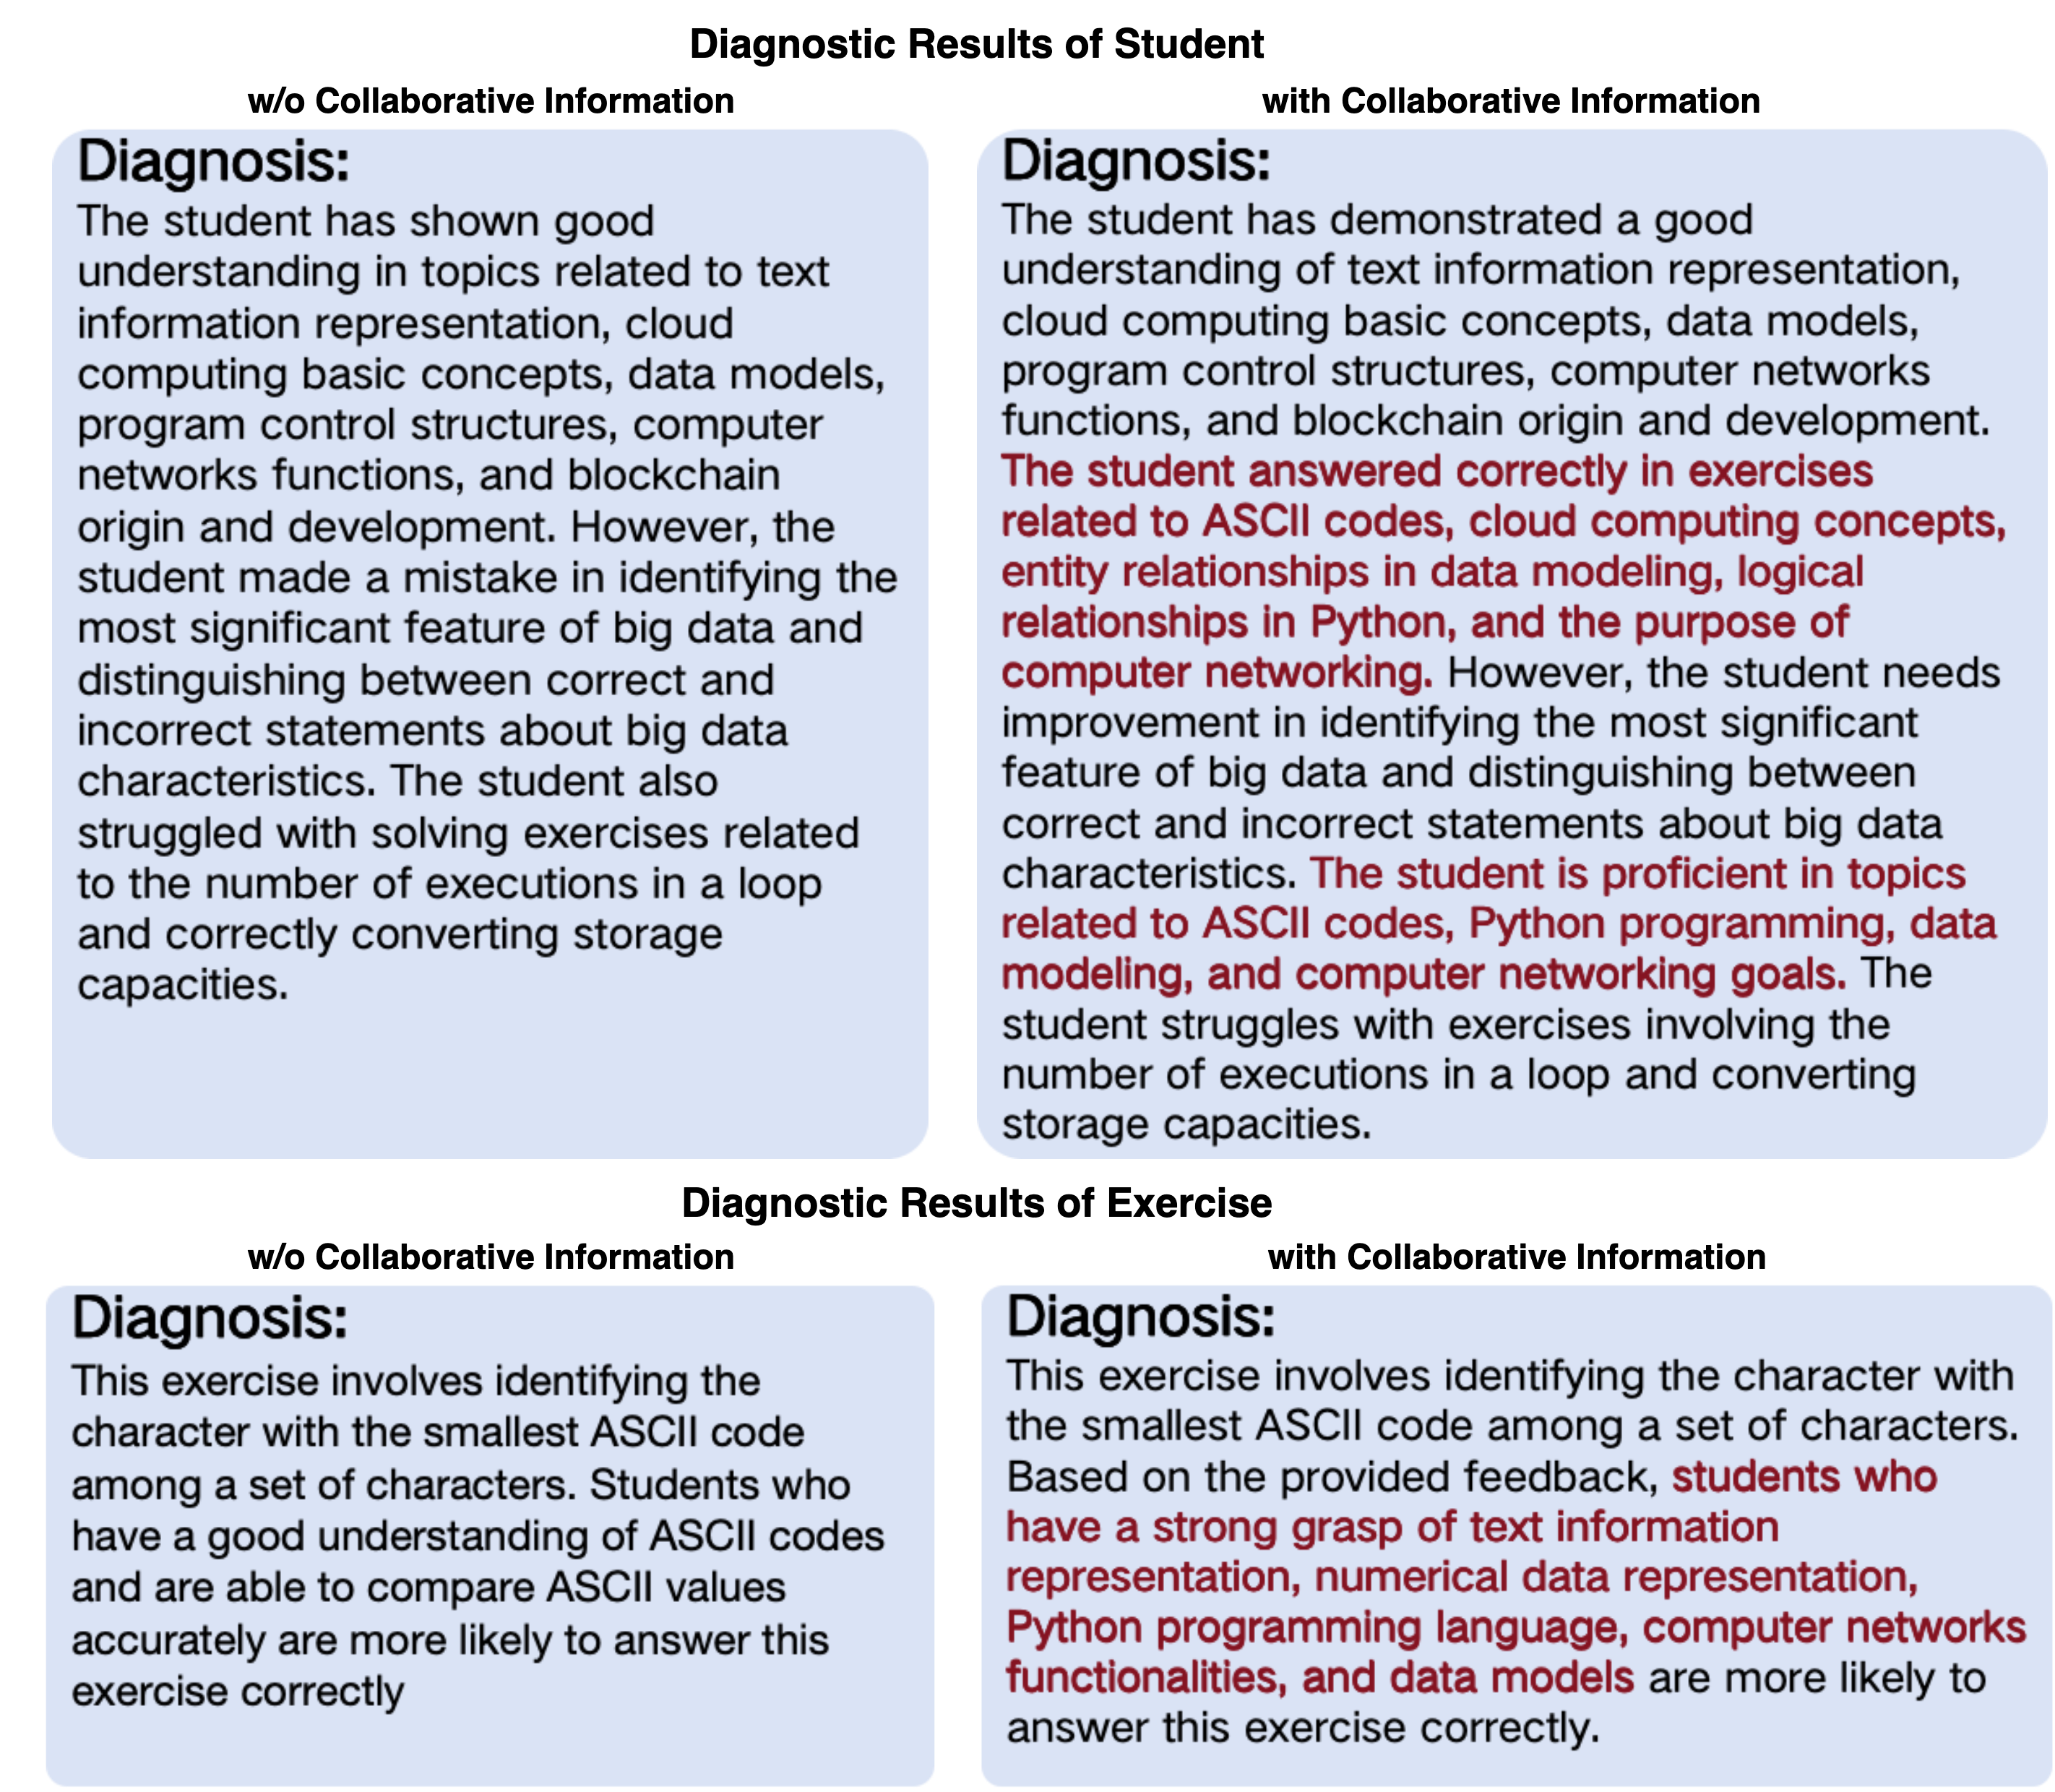}
  \caption{The example of diagnostic results of LLMs Diagnosis.}
\label{fig: diagnosis}
\end{figure*}

\begin{figure*}[!htb]
  \centering
  \includegraphics[width=0.9\linewidth]{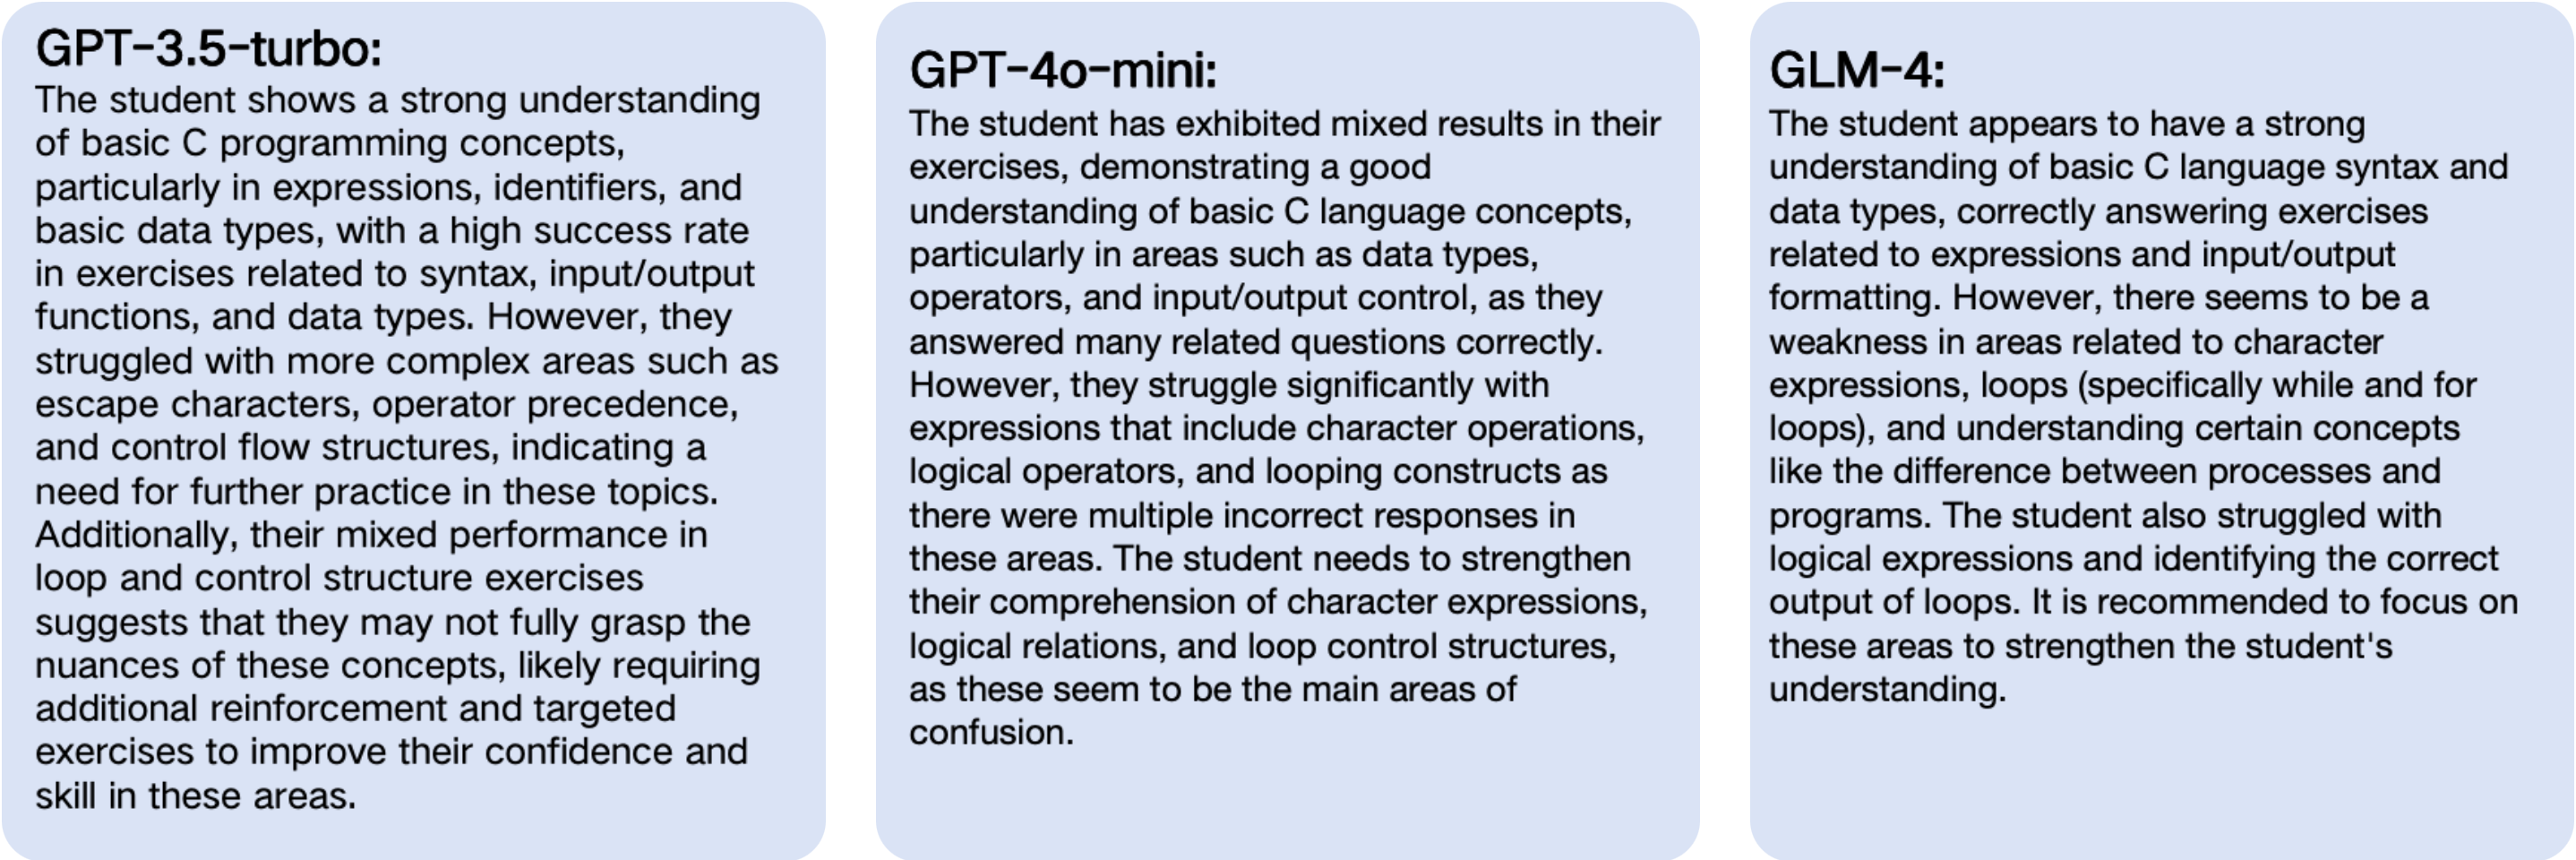}
  \caption{Diagnostic results of an example student with different LLMs.}
\label{fig: diagnosis2}
\end{figure*}

\appendix

\section{Appendix}

\subsection{Details of LLMs Diagnosis}
In this section, we provide a detailed introduction to the process of diagnosing LLMs. Using the students and exercises in the Python dataset from PTADisc as an example, we illustrate the process of diagnosis generation. Figure~\ref{fig: prompt} and Figure~\ref{fig: diagnosis} demonstrate the prompts used in this process and the examples of diagnostic results of students and exercises.

\subsubsection{Example of Used Prompts}
Figure~\ref{fig: prompt} shows the prompts we used in the Collaborative Information Collection and Diagnosis Generation processes, specifically divided into system prompts $\mathcal{M}$ and input prompts $\mathcal{P}$. The system prompt defines the role of the LLMs and introduces the format of the input prompt. It also specifies the format of the output. Here, to facilitate understanding of the LLMs, we convert the response logs into JSON format and specify that the output should also be in JSON format. To enhance the logical consistency of the LLMs' output and reduce the hallucinations, we also require them to provide reasons for their diagnostic results.
The input prompt is composed of the corresponding response logs. For the student, it includes information about the exercises they have completed. For the exercise, it includes information about the exercise itself and the completion status of all students who participated in this exercise.
Since LLMs can handle multiple languages, such as Chinese and English, the texts in the dataset can be in English or other languages. In the example shown in Figure~\ref{fig: prompt}, the information on the exercises and knowledge concepts in the PTADisc dataset is in Chinese, so we directly use Chinese to construct the input prompt.
After obtaining collaborative information, namely the overall description of students and exercises, we include this information as the profile of students and exercises in the input prompts. This allows for a more comprehensive diagnosis of both students and exercises.

\subsubsection{Comparision of Diagnostic Results}
Figure~\ref{fig: diagnosis} shows the diagnostic result of an example student and exercise Collaborative Information Collection and Diagnosis Generation, where the main difference lies in whether collaborative information is included.
From the results, it is evident that obtaining collaborative information allows for a more comprehensive diagnosis of the student's cognitive status and the attributes of the exercises.
Compared to the student, the exercise benefits significantly more from collaborative information. This is because, for the exercise, having information on all participating students allows for a more comprehensive assessment of the exercise's attributes. For the student, the information included in their response logs about the exercises they completed is usually sufficient to diagnose their cognitive status, so the addition of collaborative information does not provide a substantial improvement.

As illustrated in the figure, knowledge-enriched LLMs are capable of diagnosing both students and exercises, thereby producing comprehensive and explainable diagnostic results. Such diagnostic results can be better integrated with CDMs to achieve more accurate and comprehensive cognitive diagnoses.

\subsubsection{Comparision of Different LLMs}
\label{sec:app_llm}

\begin{table}[ht]
\centering
 %Methods with `$^{*}$' means directly using ground truth review text in the testing phase, which are not feasible in practice.

\scalebox{0.9}{
\begin{tabular}{lcccc}
\toprule
LLM & Method &  AUC  & ACC & RMSE \\ \midrule
& NCD & 0.8256 & 0.7759 & 0.3926 \\ 
\midrule
\multirow{2}{*}{GPT-3.5-turbo}& NCD-Beh & 0.8422 &  0.7928 & 0.3781 \\
& NCD-Sem & 0.8460 & 0.7963 & 0.3764\\
\midrule
\multirow{2}{*}{GPT-4o-mini} &NCD-Beh &  0.8454 & 0.7963 & 0.3744\\
&NCD-Sem &  0.8491 & 0.7981 & 0.3715 \\
\midrule
\multirow{2}{*}{GLM-4} & NCD-Beh &  0.8432 & 0.7949 & 0.3758\\
&NCD-Sem &  0.8476 & 0.7975 & 0.3749 \\
 
 \midrule
\multirow{2}{*}{Qwen2.5-72B} & NCD-Beh &  0.8407 & 0.7912 & 0.3795\\
&NCD-Sem &  0.8415 & 0.7938 & 0.3772 \\

\midrule
\multirow{2}{*}{Qwen2.5-14B} & NCD-Beh &  0.8379 & 0.7882 & 0.3813\\
&NCD-Sem &  0.8381 & 0.7906 & 0.3794 \\

 \midrule
\multirow{2}{*}{Qwen2.5-coder-7B} & NCD-Beh &  0.8342 & 0.7834 & 0.3854\\
&NCD-Sem &  0.8367 & 0.7862 & 0.3825 \\

\bottomrule 
\end{tabular}}
\caption{Different LLMs on Linux dataset.}
\label{tab:llms}
\end{table}
In this section, we replace GPT-3.5-turbo with different LLMs to measure the impact on the LLMs diagnosis process.
Specifically, we utilize OpenAI's newly released GPT-4o-mini and another popular and powerful LLM, GLM-4~\cite{glm2024chatglm} and Qwen~\cite{hui2024qwen2}, to conduct the experiments.

As demonstrated in Table~\ref{tab:llms}, using GPT-4o-mini and GLM-4 yields slightly better results. 
This is because GPT-4o-mini, a more powerful model released by OpenAI, possesses superior understanding and reasoning capabilities compared to GPT-3.5-turbo. On the other hand, GLM-4 has stronger Chinese comprehension abilities, which enhances its ability to understand the Chinese questions in the exercise. 
However, these LLMs, which also possess strong prior knowledge and reasoning abilities, have only slight differences in their capabilities. As a result, the diagnostic outcomes may not show significant variations, which explains why the final diagnostic results of different LLMs do not differ substantially.
%For more detailed diagnostic examples, please refer to Appendix.

To clearly demonstrate the differences in diagnostics generated by various LLMs, we selected the diagnostic result of a specific student as an example for display.
As shown in Figure~\ref{fig: diagnosis2}, the three LLMs provided diagnoses of the student's cognitive state from different perspectives.
It is obvious that their diagnoses about the student's understanding of specific knowledge concepts, such as `syntax', `input/output control', and `loop', are accurate and comprehensive. 
At the same time, these LLMs can leverage their capabilities to understand and reason about this information, resulting in varied summaries and generalizations of the knowledge points rather than simple listings. Additionally, LLMs can supplement the knowledge points based on the information contained in the exercise content, thereby obtaining a more fine-grained understanding of the student's cognitive status.

\subsection{Details of Baseline Models}
\noindent\textbf{IRT}~\cite{lord1952theory} is a basic CDM that represents students and exercises as unidimensional traits and captures their interactions utilizing a linear function.

\noindent\textbf{MIRT}~\cite{reckase200618} expands the traits of students and exercises in IRT to multiple dimensions.

\noindent\textbf{NCD}~\cite{wang2020neural} utilizes deep neural networks to model the interactions between students and exercises.

\noindent\textbf{DINA}~\cite{de2009dina} models the factors of students and exercises as binary vectors, including guessing and slipping parameters to evaluate performance.

\noindent\textbf{RCD}~\cite{gao2021rcd} captures the relationships between students, exercises, and knowledge concepts using Graph Convolutional Networks.

\noindent\textbf{SCD}~\cite{wang2023self} utilize self-supervised learning to enhance the modeling of students and exercises in graph-based cognitive diagnosis, alleviating the long-tail distribution problem.

\noindent\textbf{ACD}~\cite{wang2024boosting} takes into account the emotional state of students while answering questions, designs an emotional cognition module, and combines it with traditional cognitive models, achieving good results.
